# Supplementary material for: Reliability Validation of Learning Enabled Vehicle Tracking
Source: arXiv:2002.02424 source file (2020-02-06)
Supplement: Supplementary file 1 [file appendix.tex]

\begin{figure*}[h]
\centering
\includegraphics[width=12cm]{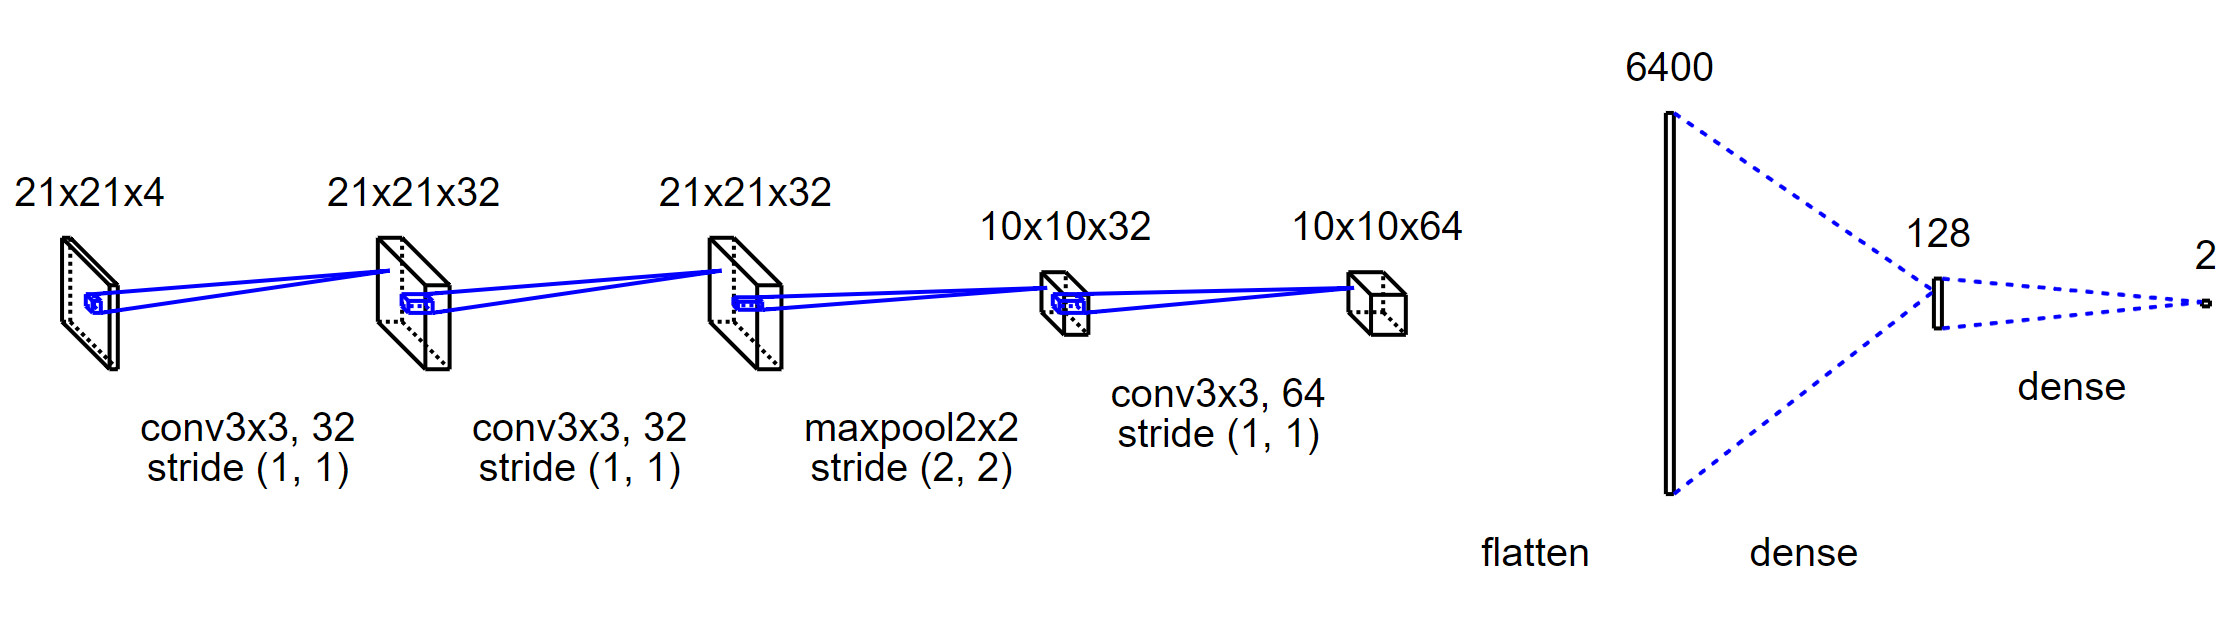}
\caption{The architecture of the classification CNN described in Section~\ref{sec:refinement}. \label{fig:CNN-arch1}}
\end{figure*}

\begin{figure*}[h]
\centering
\includegraphics[width=12cm]{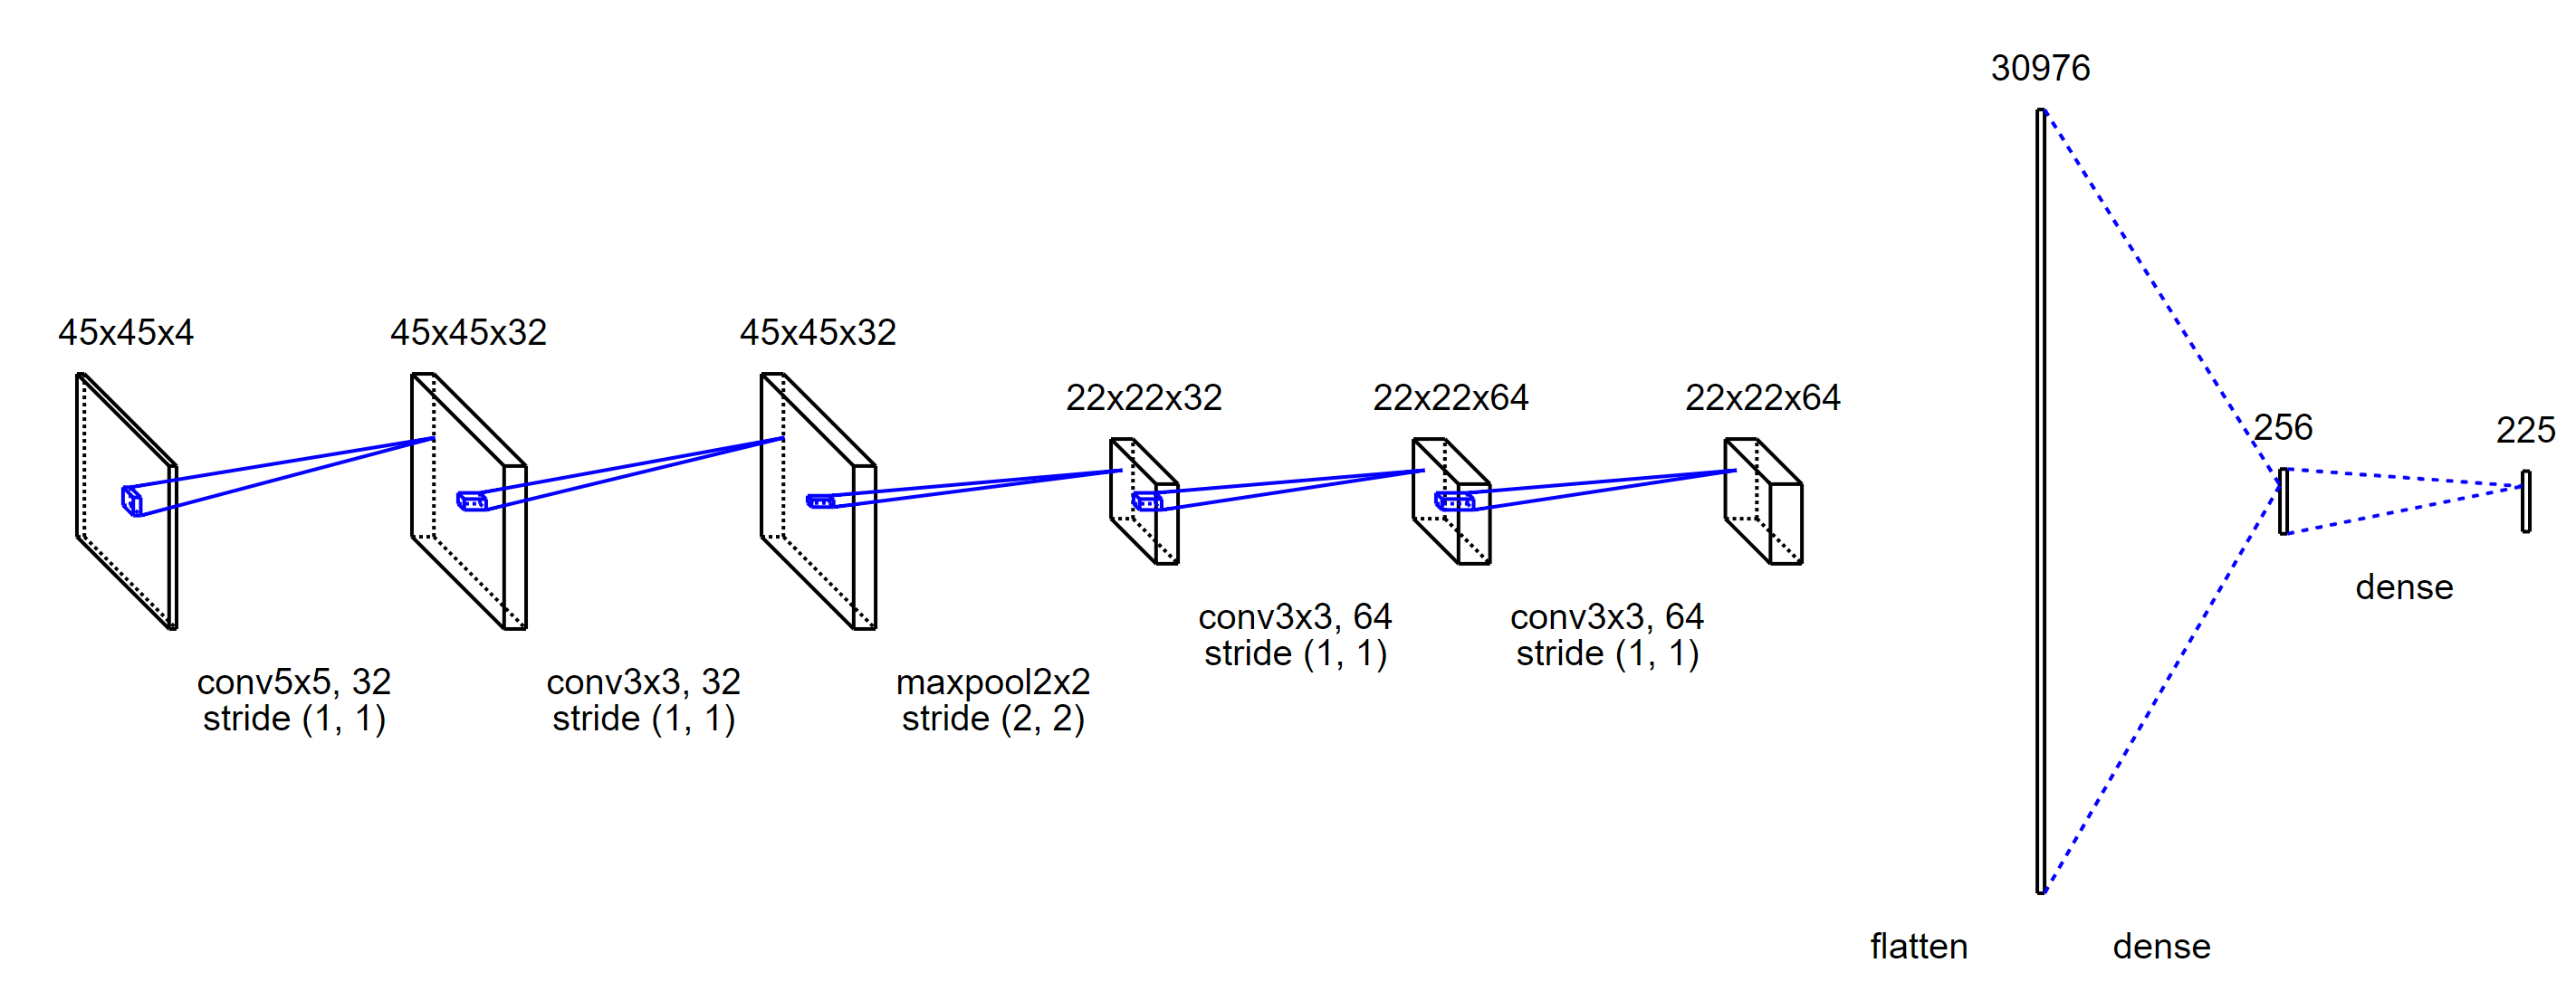}
\caption{The architecture of the regression CNN described in Section~\ref{sec:position}.\label{fig:CNN-arch2}}
\end{figure*}
